# Supplementary material for: NavTuner: Learning a Scene-Sensitive Family of Navigation Policies
Source: arXiv:2103.01464 source file (2021-03-02)
Supplement: Supplementary file 1 [file appendix.tex]

\begin{table*}[t]
	\caption{Evaluation Results for Maze Environments}
	\label{tab:results}
	\centering
	\begin{tabular}{|c|c|c|c|c|c|c|c|c|c|c|}
		\hline
		&\multirow{2}{*}{Default Value} &\multirow{2}{*}{Best Value} & \multicolumn{3}{c|}{Classifier} & \multicolumn{3}{c|}{Regressor} & \multicolumn{2}{c|}{DQN} \\\cline{4-11}
		&&& Linear & NN & CNN & Linear & NN & CNN & Scratch & Warm Start\\\hline
		Number of Success & 67&	78&	70&	73&	74&	69&	72&	75&	81&	80\\\hline
		Path Length/m & 27.5&	24.97&	25.92&	25.29&	24.96&	26.54&	25.88&	25.15&	25.87&	25.64\\\hline
		Runtime/s & 63.3&	56.74&	62.88&	55.45&	54.05&	59.125&	58.6&	57.44&	57.85&	56.51\\\hline
	\end{tabular}
	\subcaption{Evaluation with Same Wall Setup (lookahead distance)}
	\centering
	\begin{tabular}{|c|c|c|c|c|c|c|c|c|c|c|}
		\hline
		&\multirow{2}{*}{Default Value} &\multirow{2}{*}{Best Value} & \multicolumn{3}{c|}{Classifier} & \multicolumn{3}{c|}{Regressor} & \multicolumn{2}{c|}{DQN} \\\cline{4-11}
		&&& Linear & NN & CNN & Linear & NN & CNN & Scratch & Warm Start\\\hline
		Number of Success & 68&	75&	69&	71&	74&	69&	71&	73&	80&	80 \\\hline
		Path Length/m & 26.17&	24.71&	25.90&	25.42&	24.93&	25.76&	25.28&	24.84&	25.23&	25.11\\\hline
		Runtime/s & 59.68&	54.16&	60.19&	51.38&	53.60&	56.88&	55.73&	53.10&	55.54&	54.45\\\hline
	\end{tabular}
	\subcaption{Evaluation with Different Wall Setup (lookahead distance)}
	\centering
	\begin{tabular}{|c|c|c|c|c|c|c|c|c|c|c|}
		\hline
		&\multirow{2}{*}{Default Value} &\multirow{2}{*}{Best Value} & \multicolumn{3}{c|}{Classifier} & \multicolumn{3}{c|}{Regressor} & \multicolumn{2}{c|}{DQN} \\\cline{4-11}
		&&& Linear & NN & CNN & Linear & NN & CNN & Scratch & Warm Start\\\hline
		Number of Success & 70&	82&	73&	75&	80&	74&	77&	79&	84&	82\\\hline
		Path Length/m & 27.8&	25.85&	27.67&	27.09&	26.69&	27.29&	26.88&	26.4&	25.97&	25.68\\\hline
		Runtime/s & 61.16	&57.92&	60.26&	58.49&	58.25&	60.46&	58.84&	58.34&	58&	56.47\\\hline
	\end{tabular}
	\subcaption{Evaluation with Same Wall Setup (global planning frequency)}
	\centering
	\begin{tabular}{|c|c|c|c|c|c|c|c|c|c|c|}
		\hline
		&\multirow{2}{*}{Default Value} &\multirow{2}{*}{Best Value} & \multicolumn{3}{c|}{Classifier} & \multicolumn{3}{c|}{Regressor} & \multicolumn{2}{c|}{DQN} \\\cline{4-11}
		&&& Linear & NN & CNN & Linear & NN & CNN & Scratch & Warm Start\\\hline
		Number of Success & 72&	76&	73&	74&	75&	73&	73	&74&	80&	77\\\hline
		Path Length/m & 27.1&	25.7&	26.39&	26.08&	25.98&	26.5&	26.27&	25.78&	25.47&	26.02\\\hline
		Runtime/s & 59.68&	54.16&	60.19&	51.38&	53.60&	56.88&	55.73&	53.10&	55.54&	54.45\\\hline
	\end{tabular}
	\subcaption{Evaluation with Same Wall Setup (two hyper-parameters together)}
	\centering
	\begin{tabular}{|c|c|c|c|c|c|c|c|c|c|c|}
		\hline
		\multicolumn{2}{|c|}{}&\multirow{2}{*}{Best Value} & \multicolumn{3}{c|}{Classifier} & \multicolumn{3}{c|}{Regressor} & \multicolumn{2}{c|}{DQN} \\\cline{4-11}
		\multicolumn{2}{|c|}{}&& Linear & NN & CNN & Linear & NN & CNN & Scratch & Warm Start\\\hline
		\multirow{2}{*}{Lookahead(Same Wall)} & Success &	11(0.16)&	3(0.04)&	6(0.09)	&7(0.10)&	2(0.03)&	5(0.07)&	8(0.12)	&13(0.19)&	12(0.18)\\\cline{2-11}
		& Path Length/m &	2.53(0.10)&	1.58(0.06)&	2.21(0.08)&	2.54(0.10)&	0.96(0.03)&	1.62(0.06)&	2.35(0.09)&	1.63(0.06)&	1.86(0.07)\\\hline
		\multirow{2}{*}{Lookahead(Diff. Wall)} & Success &	7(0.11)&	1(0.01)&	3(0.04)&	6(0.09)&	1(0.01)&	3(0.04)&	5(0.07)	&12(0.18)&	12(0.18)\\\cline{2-11}
		& Path Length/m &	1.46(0.06)&	0.27(0.01)&	0.75(0.03)&	1.24(0.04)&	0.40(0.02)	&0.89(0.03)&	1.33(0.05)&	0.94(0.04)&	1.06(0.04)\\\hline
		\multirow{2}{*}{Global Planning Freq.} & Success &	12(0.17)&	3(0.04)	&5(0.07)	&10(0.14)&	4(0.06)	&7(0.10)&	9(0.13)	&14(0.20)&	12(0.17)\\\cline{2-11}
		& Path Length/m &	1.95(0.07)	&0.13(0.01)&	0.71(0.03)&	1.11(0.04)&	0.51(0.02)&	0.92(0.03)&	1.4(0.05)&	1.83(0.07)&	2.12(0.08)\\\hline
		\multirow{2}{*}{Two Hyper-params} & Success &	4(0.06)	&1(0.01)&	2(0.03)	&3(0.04)&	1(0.01)	&1(0.01)	&2(0.04)	&8(0.11)&	5(0.07)\\\cline{2-11}
		& Path Length/m &	1.4(0.05)&	0.71(0.03)&	1.02(0.04)&	1.12(0.04)&	0.6(0.02)&	0.83(0.03)&	1.32(0.05)&	1.63(0.06)&	1.08(0.04)\\\hline
	\end{tabular}
	\subcaption{Performance Gain Compared to Default Value. Values in parenthesis are relative values}
\end{table*}

\begin{table*}[t]
	\caption{Evaluation Results for Benchmark Environments (lookahead distance)}
	\label{tab:bmrl}
	\centering
	\begin{tabular}{|c|c|c|c|c|c|c|c|c|c|}
		\hline
		&\multirow{2}{*}{Default Value}  & \multicolumn{3}{c|}{Classifier} & \multicolumn{3}{c|}{Regressor} & \multicolumn{2}{c|}{DQN} \\\cline{3-10}
		&& Linear & NN & CNN & Linear & NN & CNN & Scratch & Warm Start\\\hline
		Number of Success & 80&	86&	87&	88&	85&	86&	88	&93&	91\\\hline
		Path Length/m & 23.12&	21.83&	21.15&	20.91&	21.72&	21.53&	20.82&	20.7&	20.56\\\hline
		Runtime/s & 44.19&	44.38&	43.56&	43.87&	44.17&	42.8&	42.25&	45.05&	44.22\\\hline
	\end{tabular}
	\subcaption{Evaluation with Campus Environment}
	\centering
	\begin{tabular}{|c|c|c|c|c|c|c|c|c|c|}
		\hline
		&\multirow{2}{*}{Default Value}  & \multicolumn{3}{c|}{Classifier} & \multicolumn{3}{c|}{Regressor} & \multicolumn{2}{c|}{DQN} \\\cline{3-10}
		&& Linear & NN & CNN & Linear & NN & CNN & Scratch & Warm Start\\\hline
		Number of Success & 81&	85&	87&	88	&85&	87&	87&	94&	92 \\\hline
		Path Length/m & 66.24&	60.24&	57.54&	56.87&	60.17&	57.11&	56.51&	54.49&	55.31\\\hline
		Runtime/s & 100.42&	96.13&	96.28&	91.24&	97.1&	94.72&	94.44&	93.19&	95.52\\\hline
	\end{tabular}
	\subcaption{Evaluation with Office Environment}
	\centering
	\begin{tabular}{|c|c|c|c|c|c|c|c|c|c|}
		\hline
		&\multirow{2}{*}{Default Value}  & \multicolumn{3}{c|}{Classifier} & \multicolumn{3}{c|}{Regressor} & \multicolumn{2}{c|}{DQN} \\\cline{3-10}
		&& Linear & NN & CNN & Linear & NN & CNN & Scratch & Warm Start\\\hline
		Number of Success & 72&	75&	77&	79&	74&	77&	78&	84	&81 \\\hline
		Path Length/m & 23.9&	22.72&	21.18&	20.88&	22.74&	21.68&	20.98&	20.02	&20.24\\\hline
		Runtime/s & 44.94&	43.98&	42.76&	41.74&	44.1&	43.86&	41.93&	41.5&	42.06\\\hline
	\end{tabular}
	\subcaption{Evaluation with Sector Environment}
\end{table*}

\begin{table*}[t]
	\caption{Evaluation Results for Benchmark Environments (global planning frequency)}
	\label{tab:bmrp}
	\centering
	\begin{tabular}{|c|c|c|c|c|c|c|c|c|c|}
		\hline
		&\multirow{2}{*}{Default Value}  & \multicolumn{3}{c|}{Classifier} & \multicolumn{3}{c|}{Regressor} & \multicolumn{2}{c|}{DQN} \\\cline{3-10}
		&& Linear & NN & CNN & Linear & NN & CNN & Scratch & Warm Start\\\hline
		Number of Success & 86&	90&	92&	94	&91&	93&	93&	100&	99\\\hline
		Path Length/m & 23.05&	21.93&	21.82&	20.79&	22.34&	21.79&	20.81&	20.88&	21.11\\\hline
		Runtime/s & 44.08&	44.94&	44.18&	42.56&	44.98&	44.17&	43.59&	42.78&	44.07\\\hline
	\end{tabular}
	\subcaption{Evaluation with Campus Environment}
	\centering
	\begin{tabular}{|c|c|c|c|c|c|c|c|c|c|}
		\hline
		&\multirow{2}{*}{Default Value}  & \multicolumn{3}{c|}{Classifier} & \multicolumn{3}{c|}{Regressor} & \multicolumn{2}{c|}{DQN} \\\cline{3-10}
		&& Linear & NN & CNN & Linear & NN & CNN & Scratch & Warm Start\\\hline
		Number of Success & 87&	93&	94&	96&	92&	94&	95&	99&	99 \\\hline
		Path Length/m & 60.38&	54.21&	53.24&	52.37&	53.65&	52.9&	51.41&	51.22&	51.31\\\hline
		Runtime/s & 97.99&	95.57&	94.72&	94.73&	95.56&	94.39&	94.74&	93.56&	92.78\\\hline
	\end{tabular}
	\subcaption{Evaluation with Office Environment}
	\centering
	\begin{tabular}{|c|c|c|c|c|c|c|c|c|c|}
		\hline
		&\multirow{2}{*}{Default Value}  & \multicolumn{3}{c|}{Classifier} & \multicolumn{3}{c|}{Regressor} & \multicolumn{2}{c|}{DQN} \\\cline{3-10}
		&& Linear & NN & CNN & Linear & NN & CNN & Scratch & Warm Start\\\hline
		Number of Success & 74	&77&	79	&82&	78&	80&	83&	86&	85 \\\hline
		Path Length/m & 22.5&	21.38&	20.01&	18.98&	21.62&	20.24&	19.4&	17.74&	17.3\\\hline
		Runtime/s & 43.72&	42.7&	43.16&	42.32&	40.92&	43.64&	44.38&	41.14&	40.41\\\hline
	\end{tabular}
	\subcaption{Evaluation with Sector Environment}
\end{table*}

\begin{table*}[t]
	\caption{Evaluation Results for Benchmark Environments (two hyper-parameters together)}
	\label{tab:bmrd}
	\centering
	\begin{tabular}{|c|c|c|c|c|c|c|c|c|c|}
		\hline
		&\multirow{2}{*}{Default Value}  & \multicolumn{3}{c|}{Classifier} & \multicolumn{3}{c|}{Regressor} & \multicolumn{2}{c|}{DQN} \\\cline{3-10}
		&& Linear & NN & CNN & Linear & NN & CNN & Scratch & Warm Start\\\hline
		Number of Success & 81&	88&	89&	91	&87&	87&	88&	95&	94\\\hline
		Path Length/m & 25.75&	25.11&	24.18&	23.93&	25.4&	24.71&	23.91&	23.09&	23.45\\\hline
		Runtime/s & 49.58&	46.87&	46.65&	43.42&	49.76&	49.98&	42.44&	43.88	&49.02\\\hline
	\end{tabular}
	\subcaption{Evaluation with Campus Environment}
	\centering
	\begin{tabular}{|c|c|c|c|c|c|c|c|c|c|}
		\hline
		&\multirow{2}{*}{Default Value}  & \multicolumn{3}{c|}{Classifier} & \multicolumn{3}{c|}{Regressor} & \multicolumn{2}{c|}{DQN} \\\cline{3-10}
		&& Linear & NN & CNN & Linear & NN & CNN & Scratch & Warm Start\\\hline
		Number of Success & 83&	87	&88&	90&	87&	89&	89&	95&	94 \\\hline
		Path Length/m & 62	&56.33&	54.93&	53.63&	55.99&	54.59&	53.92&	51.93&	51.23\\\hline
		Runtime/s & 99.01&	95.19&	94.69&	94.53&	96.07&	94.91&	94.63&	95.45&	94.83\\\hline
	\end{tabular}
	\subcaption{Evaluation with Office Environment}
	\centering
	\begin{tabular}{|c|c|c|c|c|c|c|c|c|c|}
		\hline
		&\multirow{2}{*}{Default Value}  & \multicolumn{3}{c|}{Classifier} & \multicolumn{3}{c|}{Regressor} & \multicolumn{2}{c|}{DQN} \\\cline{3-10}
		&& Linear & NN & CNN & Linear & NN & CNN & Scratch & Warm Start\\\hline
		Number of Success & 70	&72&	74&	75&	73	&74&	76&	83&	82 \\\hline
		Path Length/m & 24.84&	23.5&	22.9&	21.84&	23.3&	22.62&	21.98&	20.68&	20.5\\\hline
		Runtime/s & 43.78&	44.74&	43.72	&42.3&	45.66&	44.6&	43.18&	45.64&	44.28\\\hline
	\end{tabular}
	\subcaption{Evaluation with Sector Environment}
\end{table*}

\begin{table*}[t]
	\centering
	\begin{tabular}{|c|c|c|c|c|c|c|c|c|c|c|}
		\hline
		\multicolumn{2}{|c|}{} & \multicolumn{3}{c|}{Classifier} & \multicolumn{3}{c|}{Regressor} & \multicolumn{2}{c|}{DQN} \\\cline{3-10}
		\multicolumn{2}{|c|}{}& Linear & NN & CNN & Linear & NN & CNN & Scratch & Warm Start\\\hline
		\multirow{2}{*}{Lookahead} & Success &	4.33&	6&	7.33&	3.67&	5.67&	6.67&	12.67&	10.33\\\cline{2-10}
		& Path Length/m &	2.82&	4.46&	4.87&	2.88&	4.31&	4.98&	6.02&	5.72\\\hline
		\multirow{2}{*}{Global Planning Freq.} & Success &	4.33&	6&	8.33&	4.67&	6.67&	8&	12.67&	12\\\cline{2-10}
		& Path Length/m &	2.8	&3.62&	4.6&	2.77&	3.67&	4.77&	5.36&	5.4\\\hline
		\multirow{2}{*}{Two Hyper-params} & Success &	4.33&	5.67&	7.33&	4.33&	5.33&	6.33&	13&	12\\\cline{2-10}
		& Path Length/m &	2.55&	3.53&	4.4&	2.63&	3.56&	4.26&	5.63&	5.8\\\hline
	\end{tabular}
	\caption{Performance Gain Compared to Default Value. Values are average of all three benchmark scenarios}
	\label{tab:pg}
\end{table*}

\begin{figure}[h!]
	\centering
	\includegraphics[width=\linewidth]{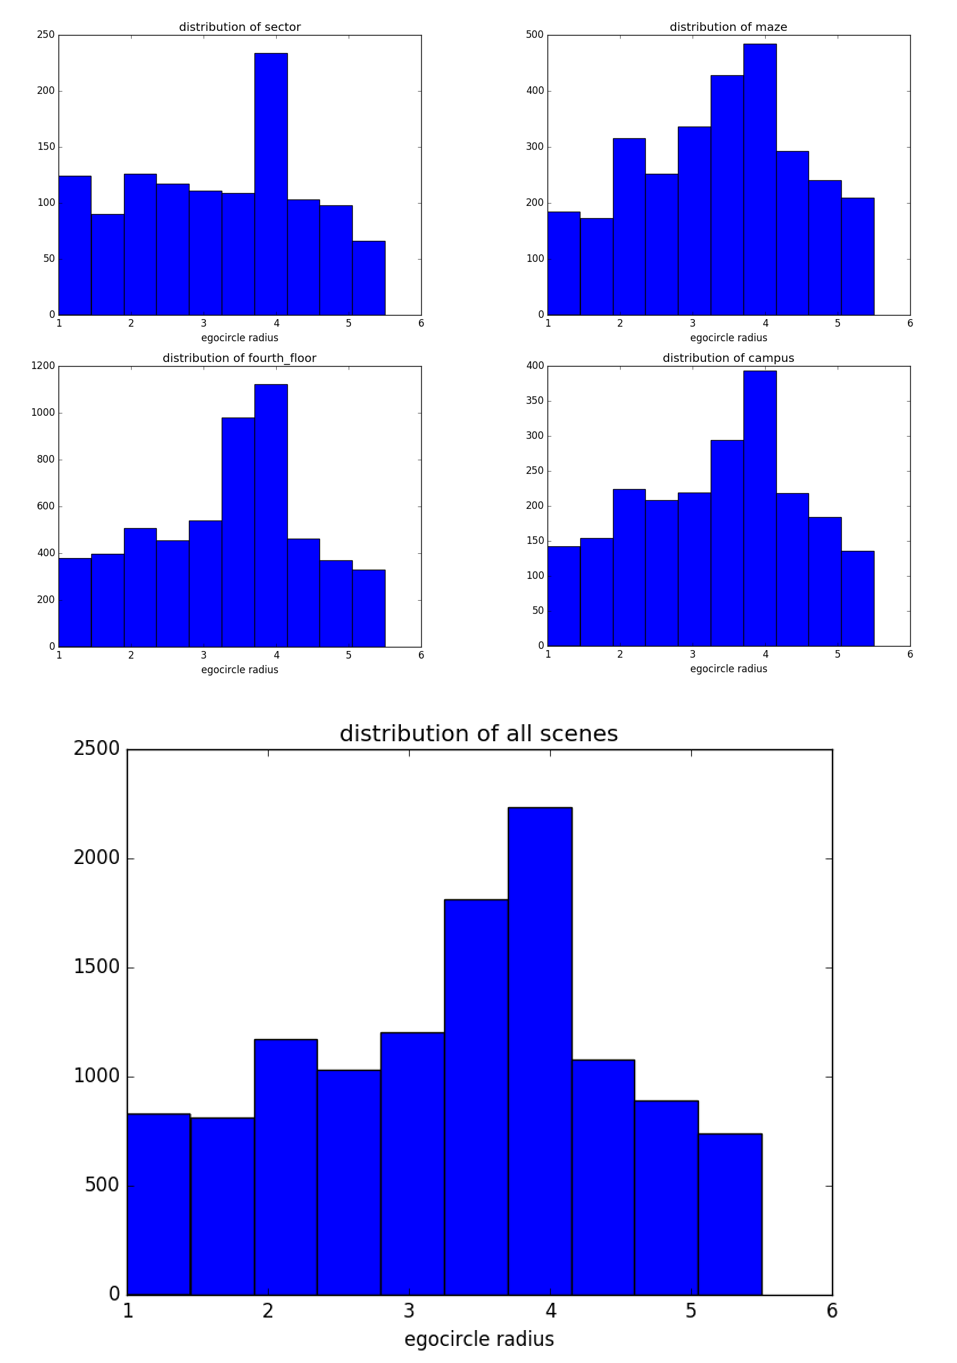}
	\caption{Distribution of Lookahead Distance}
	\label{fig:distri1}
\end{figure}
\begin{figure}
	\centering
	\includegraphics[width=\linewidth]{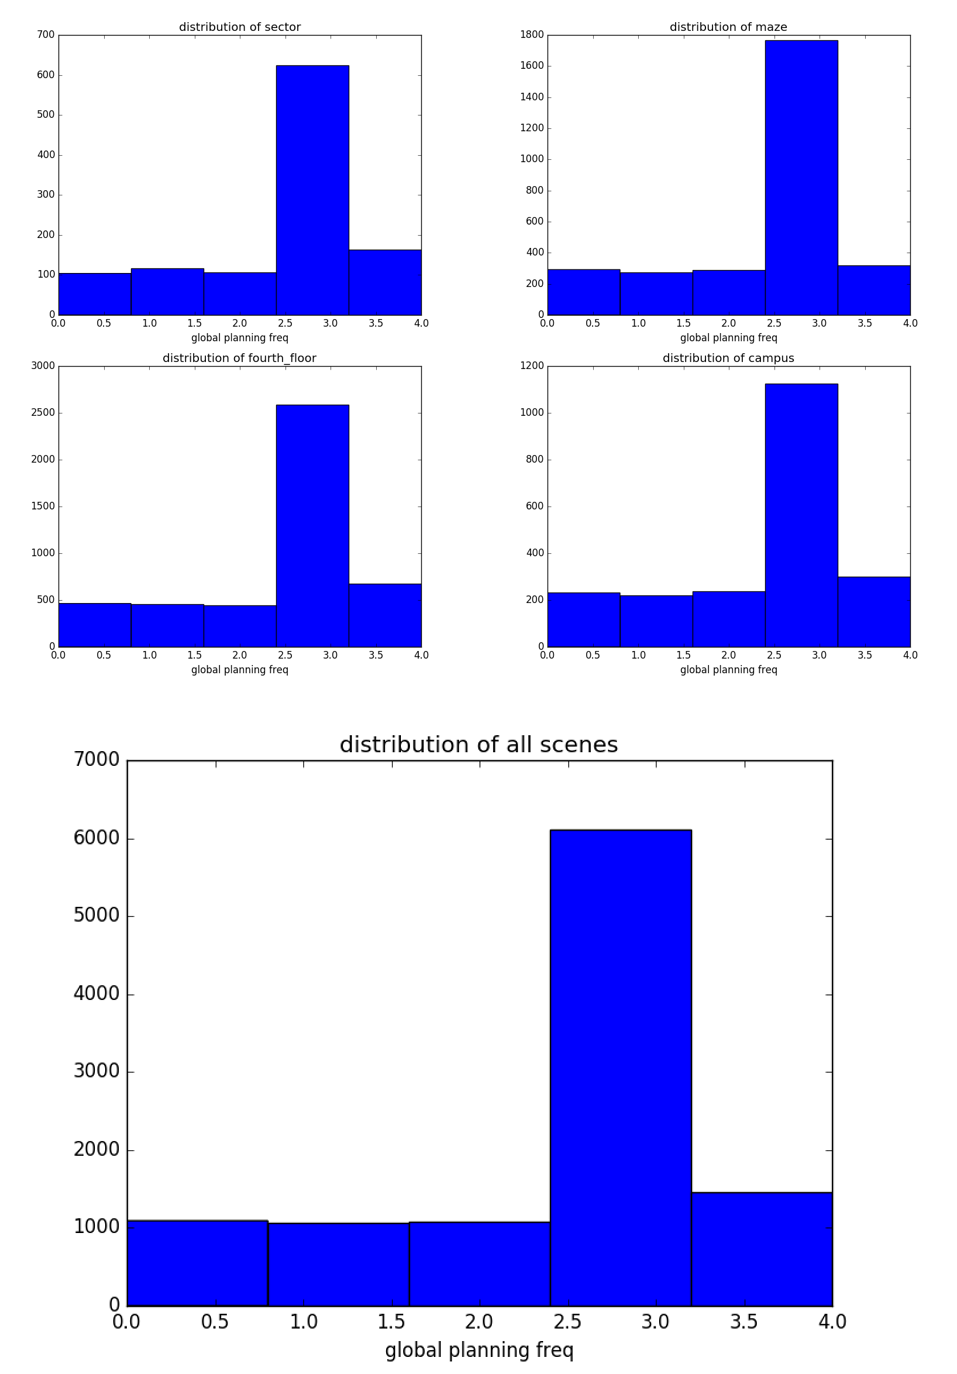}
	\caption{Distribution of Global Planning Freq.}
	\label{fig:distri2}
\end{figure}
\begin{figure}
	\centering
	\includegraphics[width=\linewidth]{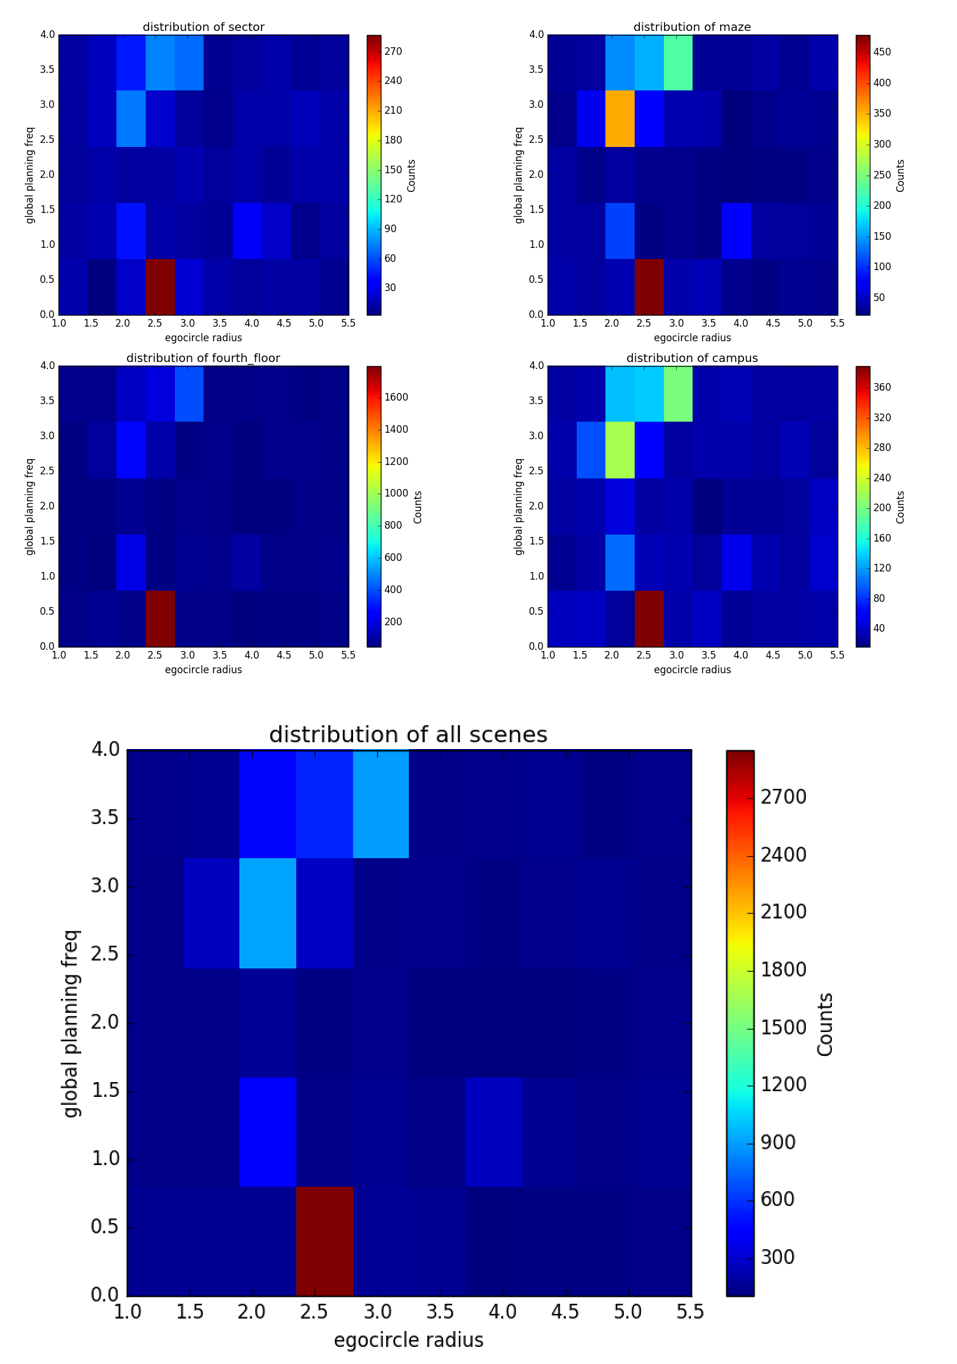}
	\caption{Distribution of Two Hyper-params}
	\label{fig:distri3}
\end{figure}

\subsubsection{Evaluation for Maze Environment}

The evaluation results for the maze environment are shown in Table \ref{tab:results}. Based on the evaluation results, we can say that the learning models have learned to predict lookahead values accordingly, so the Ego-TEB local planner with these models outperforms the basic Ego-TEB local planner. Also, the performance of the DQNs are better than the performance of the handpicked best hyper-parameter value, which may indicate that the handpicked values are not the truly optimal ones. Based on the results with the same wall setup as the training experiments and those with different wall setup, we can say that it's more likely the models are learning the local obstacle distributions instead of the wall setup.

\subsubsection{Evaluation for Benchmark Environments}

The evaluation results for the benchmark environments are shown in tables \ref{tab:bmrl}, \ref{tab:bmrp}, \ref{tab:bmrd}, and \ref{tab:pg}. From the table, we can see that the results generally follow the same pattern as those with the maze environment and the variation is more obvious, which means that the learned model can generalize well to environments not seen before.

\subsubsection{Other Findings}

Apart from the findings from the evaluation results, we also observe that the grid search result is not monotone, in other words there are multiple local optima and maybe one possible global optima. Also, based on the current grid search experiments, we find that denser scenario prefer smaller lookahead distance and larger global planning frequency. From the fact that RL models outperform our handpicked best values, we think that our handpicked best values may not be the true global optima. This can be improved by conducting further grid search with smaller grid and more experiments per grid, but the amount of improvement is not certain. We also examined the distribution of output from our DQN model trained from scratch, which is shown in figures \ref{fig:distri1}, \ref{fig:distri2}, and \ref{fig:distri3}. From the figures we can find that, RL distribution is not uniform, and instead concentrates on some specific values. The reason may be because we describe different densities as different minimum obstacle distances, so in smaller local scenarios, the expected obstacle distance may have a non-uniform distribution, and in turn a non-uniform output distribution. Another finding from the figures is that the distribution of two hyper-params does not fall in a line, or align with that of single hyper-param, which means that the two hyper-params we choose are not perpendicular to each other, and the DQN models may have converged to local optima.
